# Supplementary material for: LORD: Leveraging Open-Set Recognition with Unknown Data
Source: arXiv:2308.12584 source file (2023-08-24)

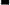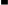

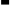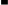

Supplement: Supplementary file 2 [file cifar100-mfmix-supmat-limit.pdf]
